# Supplementary material for: Atomic-scale nuclear spin imaging using quantum-assisted sensors in diamond
Source: arXiv:1407.3134 ancillary file (2014-07-11)
Supplement: Supplementary file 1 [file SI7.pdf]

# Atomic-scale nuclear spin imaging using quantum-assisted sensors in diamond.

## Supplementary Material

A. Ajoy[1], U. Bissbort[1,2], M.D. Lukin[3], R. Walsworth[3,4] and P. Cappellaro[1]

[1] Research Laboratory of Electronics and Department of Nuclear Science and Engineering, Massachusetts Institute of Technology, Cambridge, Massachusetts 02139, USA

[2] Singapore University of Technology and Design, 138682 Singapore

[3] Physics Department Harvard University Cambridge, Massachusetts 02138, USA

[4] Harvard-Smithsonian Center for Astrophysics and Center for Brain Science, Cambridge, Massachusetts 02138, USA

## Contents

**1 The NV center in diamond** **2**

1.1 Optical and Coherence properties of the NV spin . . . 2

**2 Simulations** **2**

2.1 CXCR4 Receptor . . . 2

2.2 Peripheral anionic site in acetylhydrolase . . . 4

**3 Position Reconstruction and Error Estimation** **6**

3.1 Reconstruction Fitting Procedure . . . 6

3.2 Alleviating the Phase Problem . . . 6

3.3 Linear Regression and Error Estimation . . . 8

3.4 Dependence on the number of inter-spin couplings . . . 10

3.5 Volume Uncertainty Dependence on Distance from NV . . . 10

3.6 Single Spin Detectability . . . 11

**4 Extension and improvements to the filtered cross-polarization sensing method** **13**

4.1 Anti-aliasing by engineered filters . . . 13

4.2 Symmetrization and robustness to power fluctuations . . . 13

**5 Comparison with other sensing schemes** **15**

**6 Geometrical pictures of the sensing schemes** **15**

6.1 Dynamical decoupling-based spin sensing . . . 16

6.2 Filtered cross-polarization spin sensing . . . 16

# 1 The NV center in diamond

## 1.1 Optical and Coherence properties of the NV spin

The Nitrogen-Vacancy (NV) center is a localized impurity in diamond, consisting of a nitrogen substitutional atom close to a vacancy (Fig. 1.A). High densities can be reached by implanting diamond with nitrogen ions and subsequently annealing to recombine the nitrogens with vacancies. Spin-dependent fluorescence, optical polarization and good coherence properties even at room temperature [? ? ] have elicited much interest in NV centers for their applications as sensors, fluorescent biomarkers and qubits. The negatively charged $NV^-$ ground state was identified as a spin triplet in ensemble ESR experiments [? ? ].

Room temperature optically detected magnetic resonance (ODMR) of a single NV spin was demonstrated in groundbreaking experiments [? ? ]. Single NV centers are addressed by optical scanning confocal microscopy with excitation at 532nm and fluorescence detection over the range 650-800nm (Fig.1.D). The NV spin state can be read under non-resonant illumination at room temperature using spin-dependent decay into metastable states (Fig. 1.B). The optical excitation conserves spin as does the direct optical decay that happens in $\approx 12$ ns. However, the $|\pm1\rangle$ states can undergo spin-orbit induced inter-system crossing [? ], decaying in $1/3^{\mathrm{rd}}$ of the cases. The metastable singlet states live for $\sim$300 ns, followed by non-radiative decay to the ground state. Thus, a NV in the $|0\rangle$ state will emit approximately 15 photons, compared to only a few for a NV in the $|\pm1\rangle$ states, yielding state discrimination by fluorescence intensity. The metastable state decays via spin-non conserving processes into the $|0\rangle$ state thereby re-orienting the spin. This reduces measurement contrast, although it allows spin polarization: laser illumination for 0.5-1$\mu$s easily achieves polarizations in excess of 95%.

The ground state of the NV electronic spin can be manipulated by on-resonance microwave fields (Fig. 1.C). The $|0\rangle$ and $|\pm1\rangle$ levels are separated by a zeros field splitting $\Delta \approx 2.87$GHz. A small magnetic field aligned with the NV axis splits the degeneracy between the $|\pm1\rangle$ levels, allowing addressing one transition at a time. The interest in the NV center stems also from its very good coherence properties. For ultra-pure diamond, the main source of decoherence is the nuclear $^{13}$C spin bath (1.1% natural abundance), which can be further suppressed in isotopically engineered diamonds [? ? ? ]. While the free precession (Ramsey signal) dephases on a fast timescale, $T_2^* \approx 2\mu$s [? ], the coherence time can be extended by using dynamical decoupling techniques [? ? ] to $T_2 \approx 600\mu$s in natural diamond [? ? ? ] and up to a few milliseconds in isotopically purified diamonds [? ? ? ]). The limiting factor is the $T_1$ relaxation process of NV centers. The process is generally slow thanks to low coupling to phonons yielding relaxation times of $T_1 \approx$5-10 ms (depending on the NV and other paramagnetic impurity density).

# 2 Simulations

## 2.1 CXCR4 Receptor

As an example of the potential of our sensing protocol, in the main text we consider the G protein-coupled chemokine receptor CXCR4 [? ] (Protein Data Bank code 3ODU). The positions of the protein atoms have been downloaded from PDB, as obtained by x-ray diffraction with 2.5Å resolution [? ]. Of particular interest

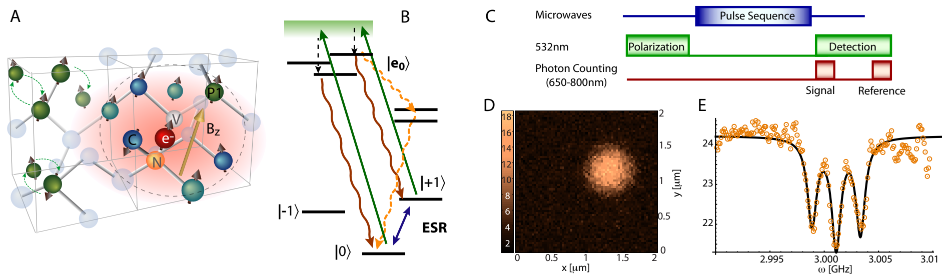


Figure 1: A) NV center in the diamond lattice and nuclear and electronic spin bath. B) Level structure of the NV center, showing spin and optical transitions responsible for spin polarization and readout, including metastable singlet states. C) Typical experiment scheme. D) Fluorescence image of NV centers by confocal spectroscopy and ODMR spectrum.

are the CXCR4 ligand-binding cavities for the small molecule IT1t, a druglike isothiourea derivative [**?** ]. We focused on the residues 183 and 185 of the binding site, assuming that the protein has been synthesized with only the desired amino acids (Arginine, ARG, for 183 and isoleucine, ILE for 185) had been $^{13}$C isotopically labeled. The protein was thus first rotated to minimize the distance from this residues to the NV center (positioned at a depth of 1.75nm), with the constraint that the whole protein should lie above the diamond surface. We then considered only the $^{13}$C of the two residues of interest (6 $^{13}$C in each residue), since all other labeled amino acid are far away and would not contribute (nor distort) the signal.

We simulated the 1D and 2D spectra recorded by the NV center using the cross-polarization method. We choose the frequency bandwidth of interest to be $1.25-4$kHz and subdivided this range in 64 bins to achieve a very smooth spectrum (note that this is not necessary in the experiments, indeed, a good spectrum is already obtained with 25 bins and this could be improved by using more advanced sampling techniques, instead of a uniform sampling). The magnetic field was set to 0.185T ($\omega_L \approx$ 2MHz) to keep the gradient time small enough and to reduce the dipolar coupling to its secular components only. The polarization time was set to $t = 720\mu$s and the gradient time to at most $T_g = 6$ms, achieved over $F = 30$ cycles. We varied the spin-lock frequency over the selected frequency range, while also varying the corresponding gradient time in order to optimally select the desired hyperfine coupling strength (see Fig. 4.A of the main text). Since the nuclear spin-spin dipolar coupling are quite strong (up to 658Hz) we considered that homonuclear decoupling was applied during both the cross-polarization and gradient evolutions. Specifically, we simulated the effects of 1 (during polarization) and 10 (during the gradient) cycles of the WAHUHA decoupling sequence [**?** ], where the time-delay between pulses was on the order of $3\mu$s. In turn, the decoupling affects the resonant frequencies as explained in the methods and reduces the effective polarization rate, thus we set the NV Rabi frequency to $\Omega = \omega_A/(2\sqrt{3})$ and the corresponding gradient time to $T_g = 2k\pi/(\omega_A/\sqrt{3}+\omega_L)$ (with $k = 400$), where $\omega_A$ is the targeted hyperfine frequency.

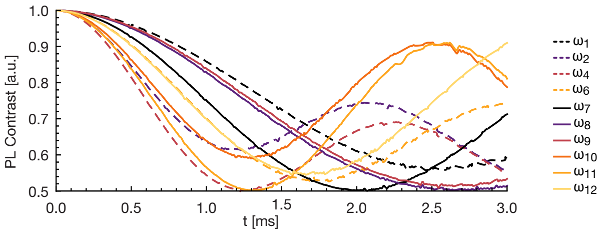


Figure 2: NV photoluminescence contrast (a.u.) as a function of the cross polarization time $t$ under rf driving at the target spin frequencies. The transverse hyperfine coupling to the target spins can be inferred with more precision from these curves. Note that the dynamics reveals additional information about the spin system: for example, driving at slightly different frequencies ($\omega_2$ and $\omega_4$, $\omega_9$ and $\omega_{10}$) one reveals the presence of additional spins, that have very similar longitudinal hyperfine coupling (see Fig. 4 of the main textfor the frequency labeling). In the 1D spectrum (Fig. 4 of the main text), the presence of these spins was only hinted to by the size of the dip at that frequency.

To obtain the 2D spectra we simulated the reverse sensing control sequence over the same frequency range and with the same parameters as the sensing/polarizing step, after letting evolve the nuclear spins for a time $300\mu$s (see Fig. 4.C of the main text). For comparison, we also show in Fig. 4.B the 2D spectrum with zero diffusion time. We note that this 2D spectrum highlights the polarization transfer in the nuclear spin network and the corresponding spatial proximity; however, the spectrum has not been optimized to extract the relevant information.

Indeed, once the spins have been identified with a 1D spectrum (Sense/Polarize step) further information about their position can be better extracted by focusing on their frequencies only. The 1D spectrum provides high precision information on the longitudinal hyperfine couplings $A_j$, thanks to the high frequency selectivity of the gradient filter. While the 1D spectrum also provides information of the transverse hyperfine couplings $B_j$, their estimated value might be less precise, if e.g. spin-spin couplings have not been precisely refocused or if there are spins with close-by $A_j$ values. A more precise estimate of the transverse hyperfine couplings can be obtained by fixing the target frequency $\omega_A = A_j$ and varying the polarization time. In order to estimate the dipole-dipole couplings, instead of considering the 2D spectrum as depicted in figure 4 of the main text, a better strategy is to only select pairs of frequencies (as determined by the 1D spectrum) and vary the mixing time. This enables following the flow of polarization from one spin to another, thus

determining their dipolar coupling. The couplings can be estimated by fitting to a model of evolution under the full dipolar Hamiltonian.

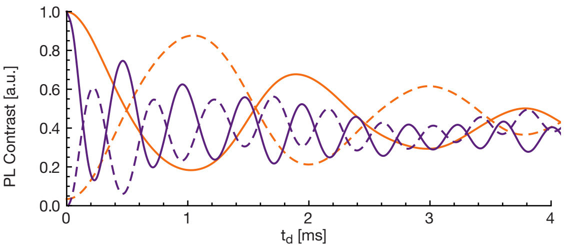


Figure 3: Normalized NV photoluminescence contrast as a function of the diffusion time $t_d$ for two pairs of excitation frequencies. The selected frequencies (for polarization and reverse sensing) excite two $^{13}$C in the 185 residue which are each strongly coupled by the dipole-dipole interaction to two other spins. Thus polarization excited with driving at 2.5kHz (violet) and 3.3kHz (orange) during the polarization step (solid lines) is transferred to other spins and read out (dashed lines) at 2.8kHz and 3.7kHz respectively, during the reverse polarization step. From the spin dynamics as a function of $t_d$ one can infer the strength of the coupling, 658Hz and 143Hz, respectively.

## 2.2 Peripheral anionic site in acetylhydrolase

In order to show the potential of the sensing scheme to provide information about a variety of molecules, we provide another example of simulated spectra.

We consider the peripheral anionic site (PAS) in acetylcholinesterase (AChE [**? ? ?** ]), a key enzyme in the nervous system. AChE binding sites are actively studied to develop targeted inhibitors that can improve cognitive abilities in Alzheimer's disease patients [**?** ]. Bivalent AChE inhibitors, which can interact with both the PAS and catalytic anionic binding sub-site, can produce more potent AD drugs, thus the PAS sub-site structure has been fully characterized and can serve as an example of how the NV-based protocol would extract information from similar, yet to be characterized, molecules.

To reconstruct the structure of PAS with the proposed scheme, we simulated the dynamics of the NV electronic spin under the action of the control sequences and the protein's nuclear spins. In the simulations we assumed that only the amino-acid TRP is $^{13}$C-labeled, thus we can focus just on the 11 $^{13}$C nuclear spins in the PAS binding site, as coupling to other spins (e.g. protons) is off-resonance. We further assumed to apply both heteronuclear and homonuclear decoupling sequences, so that the $^{13}$C linewidth is narrowed.

To obtain the 1D spectrum, we simulated the 11 $^{13}$C spins in the PAS binding site and an NV center 2nm away from it, with the [111] axis aligned around the vertical direction. The gradient time was varied from 204.6 to 204.9$\mu$s (for a maximum total gradient time of $T_g = 6$ms in $F = 30$ steps) while also varying the NV driving frequency accordingly. The polarization time was $t = 300\mu$s for the first 4, more far away, spins and $t = 180\mu$s for the other spins. The dip height is a measure of the transverse dipolar coupling $B_\perp^j$. The spectrum shows 9 dips, but it cannot resolve almost equivalent spins.

In Fig. 4 we show simulated 1D and 2D spectra for the PAS for an NV 2nm from it. Note that this corresponds to an NV only 1nm below the diamond surface (because of the AChE geometry) but this constraint could be reduced by fabricating a small diamond pillar containing the NV center. To illustrate the potential of our filtered scheme we increased the number of frequency bins to $b = 50$ in order to highlight the frequency resolution. The figure show the high frequency resolution the method can achieve as well as the additional information provided by the local diffusion of the polarization in the nuclear spin network.

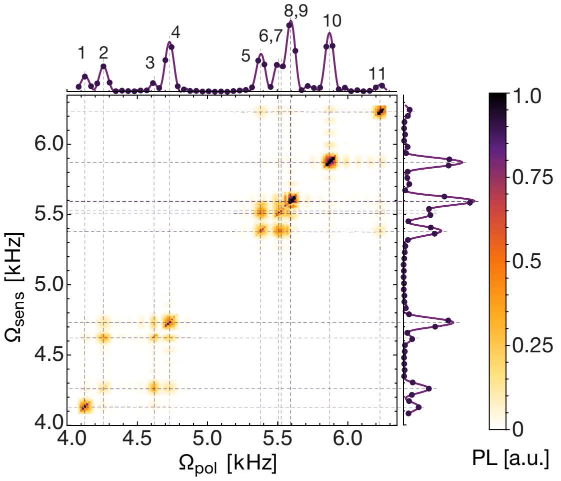


Figure 4: 1D and 2D simulated spectra for the peripheral anionic site in acetylhydrolase, obtained with the NV-based filtered sensing protocol. We plot the normalized spin-dependent photoluminescence (PL) of NV center. The 1D spectrum (on the sides of the 2D map, showing 1-PL) displays peaks when the driving frequency and the gradient time (which are swept simultaneously) match the longitudinal dipolar coupling $A^j$ of one nuclear $^{13}$C spin in the protein. The axes show the on-resonance dipolar frequency $A$ at each measurement point, while the driving frequency is $\Omega = A/2 + \omega_L$ (with Larmor frequency $\omega_L = 1.6$MHz in the simulation) and the gradient time $t_g = 2\pi/(A + \omega_L)$. The simulated 2D spectra are obtained from the proposed protocol: After polarization (obtained with the same parameters as for the 1D spectrum) the nuclear spins are let to evolve freely for $500\mu$s, allowing polarization diffusion. The polarization is then mapped back to the NV center and measured via its spin-dependent PL. The 2D spectrum shows the spreading of polarization in the spin network, as indicate from off-diagonal non-zero terms.

## 3 Position Reconstruction and Error Estimation

Here we describe the procedure used to estimate the error in the reconstructed spatial coordinates induced by errors in the coupling constants $A_j$, $B_j$, $D_{i,j}$ that would naturally arise from the sensing protocol due to finite frequency resolution and sensitivity.

We consider $N$ nuclear spins and denote their combined spherical coordinates by a $3N$-dimensional vector $\mathbf{R} = [r_1, \ldots, r_N, \vartheta_1, \ldots \vartheta_N, \varphi_1, \ldots, \varphi_N]^T$. Furthermore, we define the $L$-dimensional vector of couplings $\mathbf{P} = [A^1, \ldots, A^N, B^1, \ldots, B^N, D_{(1,2)}, \ldots, D_{(N-1,N)}]^T$, which are generally non-linear functions $\mathbf{F_P}(\mathbf{R})$ of the positions. The true positions $\overline{\mathbf{R}}$, possibly unknown, correspond to the true coupling constants $\overline{\mathbf{P}}$.

### 3.1 Reconstruction Fitting Procedure

The task of a spatial reconstruction procedure is to determine the spatial coordinates $\mathbf{R}$ of the individual spins for a given set of measured parameters $\mathbf{P}$. Here, we have to distinguish three cases:

- For $L < 3N - 1$ it is is impossible to reconstruct $\mathbf{R}$ without additional information.
- For $L = 3N - 1$ there may be a countable number of unique solutions $\mathbf{R}$, which exactly reproduce the given $\mathbf{P}$.
- For $L > 3N - 1$ the system is overdetermined. There may be no configuration compatible with all the values in $\mathbf{P}$, but one can determine an *optimal* solution from the information given.

When measuring 1D spectra only, we have the first situation; thus any scheme that does not allow measuring intra-spin couplings (as our proposed protocol) will require additional information on the molecule structure to achieve a full reconstruction.

Thanks to the polarization protocol, instead, and given the scaling of the number of couplings with $N$ (even if not all inter-spin couplings are measured), one is typically in the last regime. To find an optimal $\mathbf{R}$ for a given $\mathbf{P}$, one defines a deviation function

$$D_{\mathbf{P}}(\mathbf{R}) := \left| \sum_i \frac{\mathbf{P}_i - [\mathbf{F_P}(\mathbf{R})]_i}{\Delta P_i} \mathbf{e}_i \right|, \tag{1}$$

which is a measure (metric) in $\mathbf{P}$-space for how strongly the couplings $\mathbf{F_P}(\mathbf{R})$ resulting from a configuration $\mathbf{R}$ deviate from the given set $\mathbf{P}$. Here $|\ldots|$ is a norm defining a metric, such as the $L^p$ norm $||\mathbf{x}||_p = (\sum_j |x_j|^p)^{-1/p}$, and $\mathbf{e}_i$ is the unit vector in the $j$-th dimension. The optimal position is now determined by the value of $\mathbf{R}$ obtained by minimizing $D_{\mathbf{P}}(\mathbf{R})$. Additionally, any prior information about the magnitude of the error $\Delta P_j$ in each individual coupling (both statistical and systematic) enters as an additional ingredient in Eq. (1). This gives a higher weight to the information we know to a higher degree of accuracy and has the appealing feature that the it makes each component in the metric of $D_{\mathbf{P}}$ dimensionless. Furthermore, due to the linearity of a norm, only the relative ratios of the errors affect the result. If no perfect $\mathbf{R}$ reproducing all the measured couplings $\mathbf{P}$ exists, which is generally the case in the presence of experimental errors, the specific choice of the metric in $D_{\mathbf{P}}(\mathbf{R})$ influences the optimal position determined by this procedure, although for small errors this should not be of significance.

### 3.2 Alleviating the Phase Problem

The information obtained from a 1D spectrum allows determining the longitudinal $A^j$ and transverse $B^j$ dipolar coupling to the NV center for each nuclear spin. The knowledge of both the longitudinal and transverse couplings confines the position of each nuclear spin to a ring (and an additional to reflection on the $z = 0$ plane). The polar angle thus remains undetermined and is referred to a as the *phase problem* - also inherent to NMR spectroscopy and x-ray diffraction. Using the reverse sensing protocol gives access to the dipolar inter-spin coupling, revealing information about the relative positions of the spins. Hence, some of the polarizable spins in an entire ensemble can be used as antennas to sense other spins in their vicinity, as shown in Fig. 5(a). In an ensemble of $N$ spins there are $N(N-1)/2$ independent pairs of couplings $D_{ij}$. Hence, the number of $D$-couplings typically exceeds the number of unknown phases, allowing a reconstruction of the relative polar phases (up to a reflection on a plane through the $z$-axis) and hence the entire spatial structure. This can be substantiated by analyzing the deviation potential $D_{\mathbf{P}}(\mathbf{R})$ for two spins as a

function of the two polar angles $\varphi_1, \varphi_2$. If the coupling $D_{1,2}$ is (artificially) set to zero, $D_{\mathbf{P}}$ is independent of $\varphi_1$ and $\varphi_2$, reflecting the phase problem for both spins. If, in contrast, $D_{1,2}$ is set to a non-zero value, this independence is lifted and $D_{\mathbf{P}}$ takes on a minimum value of zero along lines of constant $|\varphi_2 - \varphi_1|$, as shown in Fig. 5(b).

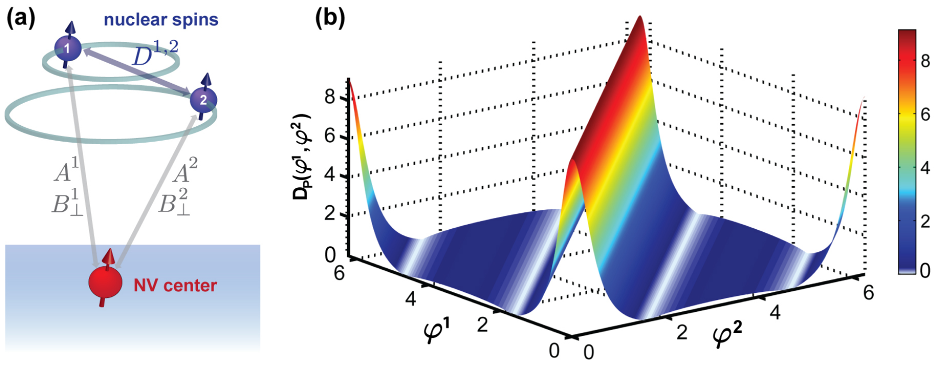


Figure 5: The deviation metric $D_{\mathbf{P}}(\varphi_1 - \varphi_2)$ for two spins at constant $z_1$, $z_2$, $r_{x,y,1}$, $r_{x,y,2}$. The knowledge of the inter-spin coupling $D_{ij}$ contains the information about the relative polar phase between the two spins, leading to a continuous minimum of $D_{\mathbf{P}} = 0$ along $|\varphi_1 - \varphi_2|$ =const.

Still, there always remains a global phase uncertainty, as a closer inspection of the couplings reveals. If the position of all spins is rotated by an arbitrary angle around the $z$-axis, all couplings remain unchanged. This is however of no significance for the proposed sensing scheme, since one is only interested in the relative coordinates of the protein spins in any structure determining procedure.

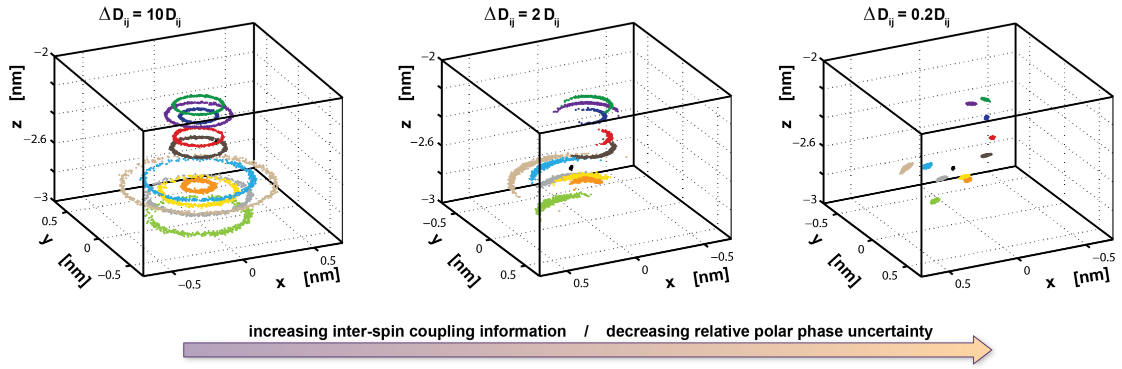


Figure 6: Alleviation of the phase problem obtained from measuring intra-spin couplings. A sequence of 3D uncertainty distributions for different relative error strength in the inter-spin couplings at $\Delta A = \Delta B = 10 Hz$, for the configuration of nuclear spins in the ligand binding site of the chemokine receptor CXCR4. For a very large error of $\Delta D_{ij} = 10 D_{ij}$ there is essentially no information available on the relative phases and the knowledge of the positions can only be restricted to radially symmetric rings, shown in the left figure. As these couplings are determined with increasing precision, this information on the relative angles (chosen relative to the spin shown in black) rotational symmetry is broken and the effective volume is reduced and eventually confined to small oval-shaped regions. The position reconstruction is performed using the procedure described in the following subsections.

### 3.3 Linear Regression and Error Estimation

The set of measured parameters $\mathbf{P} = \overline{\mathbf{P}} + \boldsymbol{\delta}\mathbf{P}$ may generally contain an error $\boldsymbol{\delta}\mathbf{P}$, composed of a statistical and a systematic component. Here we want to estimate and quantify the uncertainty induced in the position reconstruction for a given uncertainty in the measured couplings. Here $\overline{\mathbf{P}} = \mathbf{F}_{\mathbf{P}}(\overline{\mathbf{R}})$ are the (possibly unknown) true couplings, corresponding to the true positions $\overline{\mathbf{R}}$.
For sufficiently small $\boldsymbol{\delta}\mathbf{P}$, the equations $\mathbf{F}(\mathbf{R})$, where $\mathbf{R} = \overline{\mathbf{R}} + \boldsymbol{\delta}\mathbf{R}$,can be linearized around $\overline{\mathbf{R}}$

$$\mathbf{F}_{\mathbf{P}}(\mathbf{R}) = \mathbf{F}_{\mathbf{P}}(\overline{\mathbf{R}}) + J \cdot \boldsymbol{\delta}\mathbf{R} + \mathcal{O}(\boldsymbol{\delta}\mathbf{R}^2). \tag{2}$$

This yields the deviation in the parameters $\boldsymbol{\delta}\mathbf{P} = J \cdot \boldsymbol{\delta}\mathbf{R}$ for a given deviation in the positions $\boldsymbol{\delta}\mathbf{R}$ to linear order, where $J$ is the Jacobi matrix with elements $J_{i,j} = \frac{\partial[\mathbf{F}_{\mathbf{P}}(\mathbf{R})]_i}{\partial R_j}\Big|_{\overline{\mathbf{R}}}$. To estimate the position accuracy, we are however interested in the inverse case, i.e. we want to determine the deviation in the position $\boldsymbol{\delta}\mathbf{R}$ for a given deviation in the parameters $\boldsymbol{\delta}\mathbf{P}$.
For the simple case that dim($\mathbf{R}$) =dim($\mathbf{F}$), i.e. $L = 3N - 1$, the error $\boldsymbol{\delta}\mathbf{R}$ could be calculated using the inverse of the Jacobi matrix $J_{i,j} = \frac{\partial F_i}{\partial R_j}\Big|_{\overline{\mathbf{R}}}$.
However, for dim($\mathbf{F}$) >dim($\mathbf{R}$), if the number of known couplings exceeds the number of relevant spin coordinates (which is possible as soon as $N > 2$), the system of equations becomes overdetermined and does not necessarily possess a solution fulfilling all requirements. In this regime we resort to linear regression, which, for a given error $\boldsymbol{\delta}\mathbf{P}$, yields the most compatible set of $\delta\mathbf{R}$ by minimizing the deviation measure $|\boldsymbol{\delta}\mathbf{F} - J\boldsymbol{\delta}\mathbf{R}|^2$.

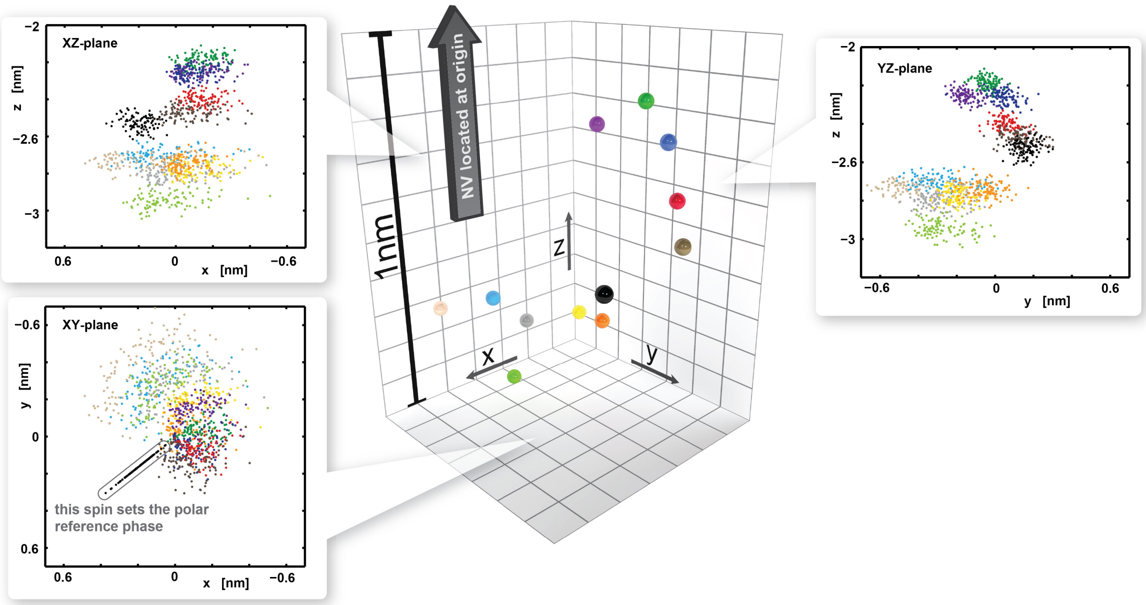


Figure 7: Accuracy of the position assignment obtained from our proposed sensing method for the $^{13}$C nuclear spins in the 183 and 185 residues of CXCR4. The spatial reconstruction uncertainty for the positions of the $^{13}$C nuclear spins is shown as scatter plots in the three planes, where the color defines the nuclear spin it refers to. Specifically, we choose the coordinates of residue 183 and 185 of the 3ODU protein [**?** ] and assume a constant error $\Delta A_j = \Delta B_j = 300$Hz and a relative error $\Delta D_{ij} = 0.5 D_{ij}$.

Here we extend upon the standard linear regression approach, which assumes an identical uncertainty for all input parameters. We present a short derivation of this extended approach and start by defining the diagonal and Hermitian matrix

$$S := \begin{pmatrix} \Delta P_1 & 0 & 0 \\ 0 & \Delta P_2 & 0 \\ 0 & 0 & \ddots \end{pmatrix}. \tag{3}$$

with the standard deviation (or more generally the uncertainty, including a possible systematic error) of the $j$-th parameter $\Delta P_j$ as the $j$-th diagonal element, the deviation of the linearized argument can be written in matrix form as

$$D_{\mathbf{P}}(\mathbf{R}) \approx \left| \sum_i \frac{\boldsymbol{\delta}\mathbf{P}_i - (J \cdot \boldsymbol{\delta}\mathbf{R})_i}{\Delta P_i} \mathbf{e}_i \right|_p = \left| S^{-1}(\boldsymbol{\delta}\mathbf{P} - (J \cdot \boldsymbol{\delta}\mathbf{R})) \right| . \tag{4}$$

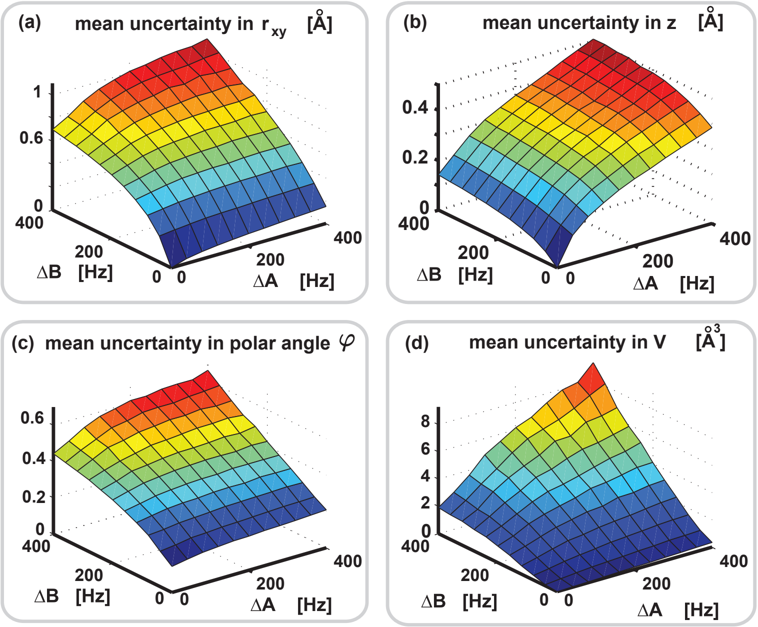


Figure 8: The uncertainty (standard deviation) induced in the cylindrical coordinates as a function of a Gaussian distributed random error with standard deviation $\Delta A$ and $\Delta B$ for the associated couplings. A relative Gaussian error $\Delta D_{ij} = 0.5 D_{ij}$ and $\Delta D_{ij}^{(bg)} = 50\text{Hz}$ is used for the inter-spin couplings. The volume corresponding to the 90th percentile, obtained from a separable integration in cylindrical coordinates, is shown in the rightmost plot.

Specifically choosing the $L^2$-norm (as is the standard procedure in linear regression), the uncertainty-weighted linear regression equations are derived by minimizing the deviation $D_{\mathbf{P}}(\mathbf{R})$ for a given set of data points $\mathbf{P}_i$, leading to the necessary condition

$$0 \stackrel{!}{=} \frac{\partial D_{\mathbf{P}}(\mathbf{R})^2}{\partial \boldsymbol{\delta}\mathbf{R}_j} \tag{5}$$

for all components $j$. If the matrix $J^\dagger S^{-2} J$ is non-singular, this can be written in matrix form as

$$\boldsymbol{\delta}\mathbf{R} = \left[ J^\dagger S^{-2} J \right]^{-1} J^\dagger S^{-2} \boldsymbol{\delta}\mathbf{P}. \tag{6}$$

This equation describes to linear order how the optimal fit, i.e. the position of the minimum of $D(\mathbf{R})$, changes if the parameters $\mathbf{P}$ deviate slightly from the true values (as induced for instance by a measurement error). To estimate the spatial uncertainty for a given uncertainty $\boldsymbol{\delta}\mathbf{F}$ in the parameters, we proceed as follows:

- From the positions $\overline{\mathbf{R}}$ of the spins (assumed to be exact), we calculate the true couplings $\mathbf{F}_{\mathbf{P}}(\overline{\mathbf{R}})$.
- We simulate the statistical measurement error by sampling each element of $\boldsymbol{\delta}\mathbf{P}$ from a Gaussian distribution with standard deviation chosen as the respective given error.
- For the resulting single realization $\mathbf{P} = \overline{\mathbf{P}} + \boldsymbol{\delta}\mathbf{P}$, we calculate the corresponding optimal position $\mathbf{R}$ using the linear regression procedure described above.
- This is repeated over many realizations, leading to distributions in the reconstructed coordinates, from which the uncertainty can be estimated and the effective uncertainty volume element can be calculated.

The positions of the spins of the protein pocket we considered and scatter plots resulting from the above simulation procedure for feasible experimental parameters are shown in Fig. 7. The uncertainty in the cylindrical coordinates and the effective 90th percentile volume is estimated from the standard deviation of the sample distributions and shown as a function of $\Delta A$ and $\Delta B$ in Fig. 8.

### 3.4 Dependence on the number of inter-spin couplings

An important feature of our proposed method is the capability to measure the inter-spin couplings $D_{ij}$, of which there are $N(N-1)/2$ for a system consisting of $N$ nuclear spins. Under realistic conditions, not all of these couplings are will be measured, nor do they have to be. Furthermore, many of these couplings will be rather small, as they fall off as $r^{-3}$, where $r$ is the distance between the respective spins.

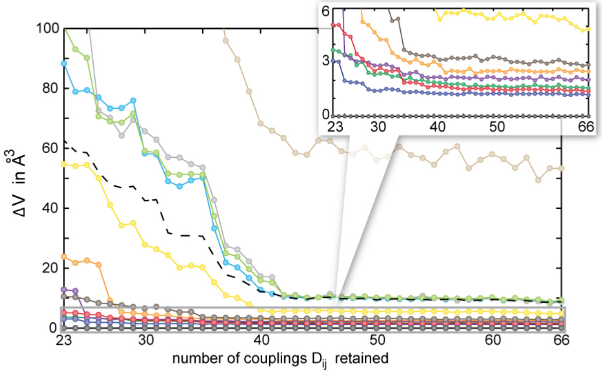


Figure 9: Volume uncertainty of individual spins (colored circles corresponding to the colors used in Fig. (7)) and average volume uncertainty (black line) as a function of the number of couplings $D_{ij}$ used in the reconstruction procedure. $\Delta A = \Delta B = 300$Hz, and a relative error of 0.5 in conjunction with a constant background uncertainty $\Delta D_{ij}^{(bg)} = 50$Hz was used for the fluctuation in the inter-spin couplings, i.e. $\Delta D_{ij} = \sqrt{(0.5 D_{ij})^2 + (50\text{Hz})^2}$. For $N = 12$ spins, there are $N(N-1)/2 = 66$ independent couplings. Here, we fixed the position of the spin shown in black in Fig. (7).

The dependence of the spins volume uncertainty on the number of measured couplings is shown in Fig. (9) for the same spatial configuration as shown in Fig. (7). The largest $D_{ij}$ in magnitude are retained for a given number of values. To account for the fact that the uncertainty in $D_{ij}$ scales with its magnitude for large $D_{ij}$, but is also bounded from below, we sample the deviation $\delta D_{ij}$ from the true value from a Gaussian with a standard deviation

$$\Delta D_{ij} = \sqrt{(\eta\, D_{ij})^2 + (\Delta D_{ij}^{(bg)})^2} \tag{7}$$

containing both a relative uncertainty $\eta$ and a constant background uncertainty $\Delta D_{ij}^{(bg)}$.

Clearly, the volume uncertainty of the individual spins decreases as the available information from an increasing number of couplings is included, featuring jumps when important couplings connecting different clusters are included. This volume uncertainty differs significantly for different spins and is primarily determined by two factors: the distance of the respective spin to the NV (which sets the uncertainty in $r_\perp$ and $z$) as well as the distance between the respective spin and the reference nuclear spin, relative to which the polar phase is specified. The volume uncertainty for the majority of the favorable spins ranges from $1.2\mathring{A}^3$ to $10\mathring{A}^3$ once the most relevant couplings have been included.

### 3.5 Volume Uncertainty Dependence on Distance from NV

Since the interaction between the nuclear spins and the NV center depends strongly on distance, this parameter – and in particular the depth of the NV below the diamond surface – is critical in determining the spatial resolution.

To estimate the volume uncertainty as a function of the distance from the NV center, we consider a simple model, where only the parameters $A$ and $B$ are measured. The uncertainty in the volume is then given by $\Delta V = \langle r \rangle\,(2\Delta r_\perp)(2\Delta z)(2\Delta\varphi) = 2\pi\,\langle r \rangle\, 4\Delta r_\perp \Delta z$, assuming the maximum uncertainty in the phase $\varphi$.

From the relationships linking $\{r_\perp, z\}$ and $\{A, B\}$, we can calculate $\Delta z$ and $\Delta r_\perp$ in the linear regime (assuming small errors $\Delta A$, $\Delta B$) as a function of the nuclear spin position. In figure 10 we plot the error uncertainty for hydrogen nuclear spins as a function of the distance from the NV.

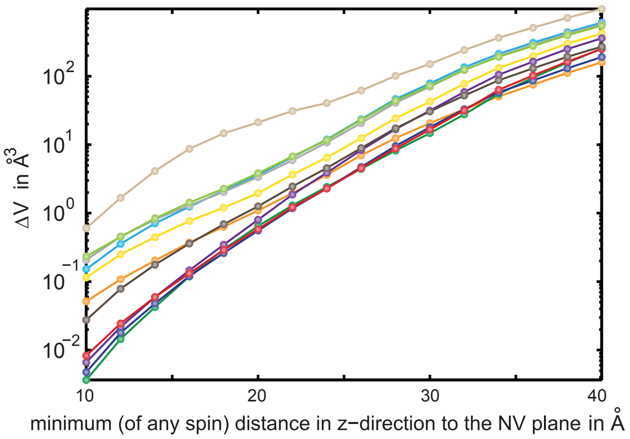


Figure 10: The volume uncertainty $\Delta V$ as a function of the distance from the NV assuming a statistical uncertainty of $\Delta D = \Delta B$=300Hz and $\Delta D = \sqrt{(D/2)^2 + (50Hz)^2}$. The NV is assumed to be aligned along the z axis ([111] crystal) and at the origin of the coordinate axes. The color coding with respect to the spins is identical to the plots above, and as shown in Fig.7.

### 3.6 Single Spin Detectability

Let us first consider the sensing capabilities for a single spin, for which case distinguishability issues do not arise. The sensing volume is given by the set of all spatially accessible points above the diamond surface, for which $B_\perp(\mathbf{r}) > \Delta B_\perp$, i.e. where the peak height is larger than the error and thus identifiable as a peak. The value of the coupling $A$, which sets the peak's position, does not affect its detectability in the case of a single spin. For both possible NV orientations [111] and [001], the dipolar coupling constants and the single spin sensing volumes are shown in (a,b) and (c) of Fig.11 and Fig.12 respectively.

Above, we have considered the detectability of a single spin. With the presence of multiple spins in the potential sensing volume, ambiguities may arise if different spins have a very similar coupling $A$, making them indistinguishable within a single spectrum. Clearly, the occurrence of such a case depends on the specific spatial configuration at hand. For the general case, the distinguishability can at best be quantified in a statistical sense, i.e. for random spatial distributions of the spins, what is the probability that the two spins are indistinguishable and how does this depend on the distance of the spins from the NV. To give quantitative insight to this question, we analyze the probability that two randomly chosen spins are distinguishable for the typical NV orientations. Furthermore, we include the dependence of the distinguishability on the distance to the NV by the following procedure: For a given distance $z$ of the plane in the $x$-$y$-direction, the position of the first spin is randomly sampled in this plane. If it is detectable, i.e. if its coupling $B$ at that position is larger than the threshold uncertainty $\Delta B$, it is accepted, otherwise the procedure is repeated. Once a valid spin in the plane has been chosen, the position of the second spin is randomly sampled from the entire volume above the plane at height $z$. For every coordinate, it is checked analogously if the spin is detectable and the procedure is again repeated until a valid detectable position has been found. Once two valid positions have been found, it is checked whether the two spins are distinguishable, i.e. whether their values of $A$, defining the peaks' positions on the frequency axis, are sufficiently different to be identified as separate peaks. This criterion is chosen as $|A^{(1)} - A^{(2)}| > \Delta A$. This Monte Carlo sampling scheme thus yields the probability that two randomly chosen spins (assuming an a priori constant spatial probability distribution) lead to independent, clearly resolved peaks, which can be distinguished by eye. This probability is shown as a function of the inter-spin separation and the minimum distance of the two spins to the NV for the two different NV orientations in FIG.11 and FIG.12 (d).

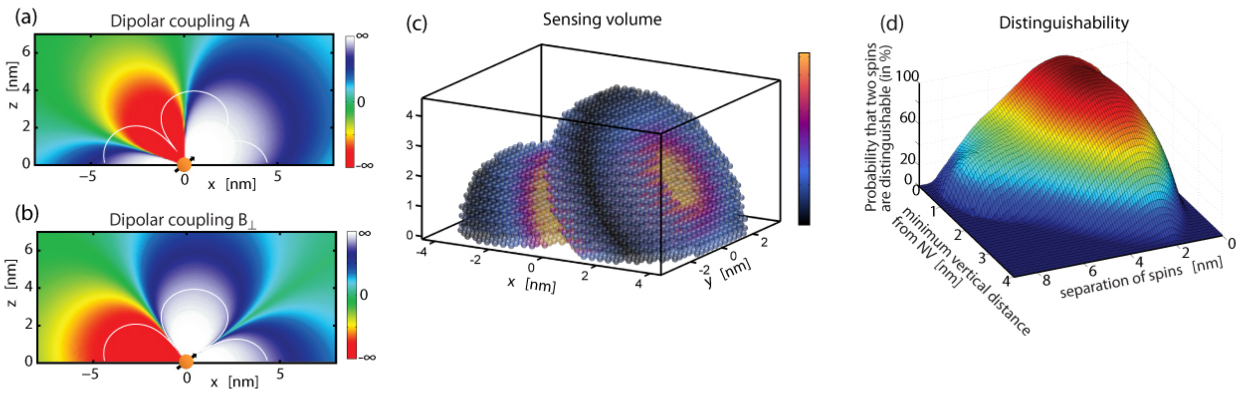


Figure 11: **Sensing Volume** – For a NV oriented in the $\sqrt{2}\mathbf{e}_x + \mathbf{e}_z$ direction (a) and (b) show the dipolar coupling constants for a $^{13}$C spin in the $y = 0$ plane as a function of distance from the NV, which is located at the origin. The diamond surface is assumed to be parallel to the $x$-$y$-plane (i.e. of the [001] type) at the $z$-value of the NV implantation height. The sensing volume, within which a single spin can be directly detected, is given by the 3D volume within which the dipolar coupling constant $B_\perp$ is of the order or larger than the uncertainty $|B_\perp| \geq \Delta B_\perp$. This sensing volume is given by the area bounded by the white lines in (a) and (b) and the structure of the 3D sensing volume is explicitly shown in (c), where the spatial dependence of the coupling $A$ is color coded. Subfigure (d) shows the a priori two-spin distinguishability (i.e. without utilizing an additional external magnetic field) as a function of the distance from the NV and the inter-spin separation. We assume an uncertainty of $\Delta A = \Delta B = 300\text{Hz} \cdot h$.

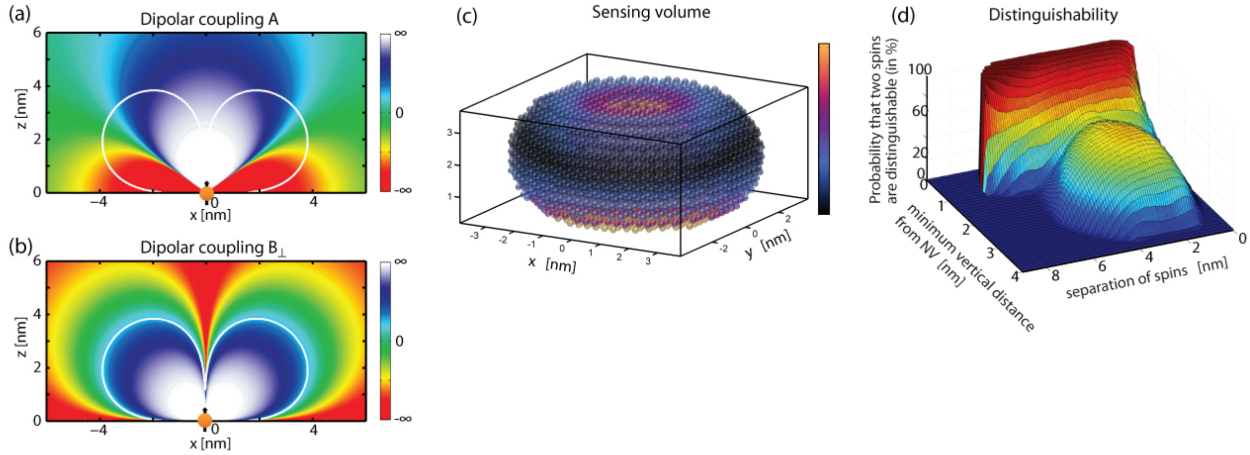


Figure 12: **Sensing Volume** – The same quantities as in Fig.11 are shown with the difference that the NV is oriented in the $\mathbf{e}_z$ direction, i.e. the diamond is of the [111] type.

# 4 Extension and improvements to the filtered cross-polarization sensing method

## 4.1 Anti-aliasing by engineered filters

The filtered sensing method achieves high spatial resolution thanks to the longer evolution times afforded by using the nuclear ancillary spin. Indeed, the filter linewidth scale as $\delta A \sim 1/(Ft_g)$. Unfortunately, the improvement in resolution comes at the cost of a reduced bandwidth which also scales as $\Delta A \sim 1/t_g$. Note that in principle since we sweep the Rabi frequency $\Omega$ in the Hartmann-Hahn sensing experiments, the sensing bandwidth is infinite. However, the "bandwidth" we shall be concerned with here is that of the sensing filter – which becomes relevant if for instance $\Omega$ is kept constant and the filter period alone is swept to sense over some frequency range. We can however overcome this resolution-bandwidth tradeoff by employing a dynamical implementation of an anti-aliasing filter.

Aliasing occurs due to the periodicity of the filter $\mathcal{G}$ over different spectral regions $\Delta A$. Here we propose a novel strategy for anti-aliasing methods that can beat this aliasing problem and boost the effective sensing bandwidth while still maintaining the high resolution afforded by the filter. The method involves making the maxima of the filter dependent on the spectral region number $m = \omega t_g/(2\pi)$, so that peaks belonging to different spectral region can be distinguished, even when they are folded over. Our approach is to introduce a slow modulation of the filter, with frequency $f_a$, thus increasing by a factor $f_a$ the bandwidth.

Fig. 13 shows the construction of the anti-aliasing filter. In one cycle, we employ $F$ cycles of $M$ alternating blocks of polarization driving with periods $\{t_k/F\}$ and free evolution with delays $\{t_{gk}\}$, with $F\sum_{k=1}^{M} t_{gk} = T_g = 2\pi F/\omega_j$. Consider for simplicity a single nuclear spin. One cycle of the sequence gives the propagator

$$\begin{aligned} U &= e^{i\omega_j I_z t_g}\left[e^{i\sum_{k=1}^{M} t_{gk}\omega_j I_z} e^{-iHt_{M-1}/F} e^{-i\sum_{k=1}^{M} t_{gk}\omega_j I_z}\right] \\ &\times \left[e^{i(t_{g1}+t_{g2})\omega_j I_z} e^{-iHt_2/F} e^{-i(t_{g1}+t_{g2})\omega_j I_z}\right]\cdots \\ &\times \left[e^{it_{g1}\omega_j I_z} e^{-iHt_1/F} e^{-it_{g1}\omega_j I_z}\right] e^{-iHt_0/F} \end{aligned} \quad (8)$$

Taking the zeroth order average Hamiltonian approximation, and considering $F$ cycles we obtain an effective Hamiltonian

$$\overline{H} = \Omega S_x + \omega_j I_z + \frac{B_\perp}{2}\mathcal{A}(\omega_j)\mathcal{G}(\omega_j) S_z I_x \quad (9)$$

with the filter

$$\mathcal{A}(\omega_j)\,\mathcal{G}(\omega_j) = \frac{1}{F}\left(\sum_{m=1}^{M} t_m e^{i\sum_{k=1}^{m} t_{gk}\omega_j}\right)\left(\sum_{k=0}^{F-1} e^{ikt_{gj}\omega_j}\right) \quad (10)$$

The function $\mathcal{A}$ thus modulates the grating $\mathcal{G}$ and its parameters (the timings $\{t_k, t_{gk}\}$) can be set to achieve anti-aliasing. For example, in Fig.13 we set $M = 3$, $t_{gk} = t_g/5\{1, 1, 0\}$ and $t_k = t\{0.4472, 0.4472, 0.7236\}$ to engineer zeros at two consecutive positions of $\mathcal{G}_j$ maxima. This provides a sharp contrast in the amplitude of the filter, and allows one to easily discern aliased peaks. The tradeoff is a loss of 37% in the filter peak amplitude, but with an increases of the sensing bandwidth by a factor 5 (the periodicity of the function $\mathcal{A}$).

## 4.2 Symmetrization and robustness to power fluctuations

The zeroth order average Hamiltonian approximation can be made accurate to first order if the toggling frame Hamiltonians are mirror anti-symmetric with respect to the center of the sequence in time. We

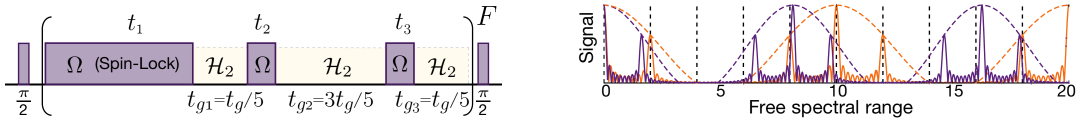


Figure 13: Anti-aliasing filter. (a) The engineered filter sequence consists of $F$ cycles of unequal time-blocks of polarization driving (for times $t_k$) and gradient evolution ($t_{gk}$). The timings are chosen to engineer a slow envelope modulation of the grating. (b) Dynamic filters for two frequencies $\omega_j$ differing by the unmodulated filter bandwidth. Under the anti-aliasing sequence, the peak heights become a function of the spectral range number $m$ and it is possible to distinguish aliased peaks from their amplitudes. The filter bandwidth is now effectively extended to the period of $\mathcal{A}$ (dashed lines).

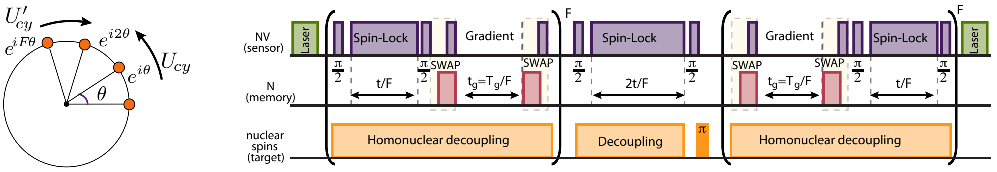


Figure 14: Symmetrized cross-polarization sequence. Left: Phasor representation of the symmetrization. In order to make the toggling frame Hamiltonians mirror antisymmetric, it is necessary to concatenate the normal propagator $U_{cy}$, which produces the grating filter $\mathcal{G}_j$, with ,an effective propagator in the opposite direction $U'_{cy}$ producing $\mathcal{G}'_j$. Here we denote the phases of each term of $\mathcal{G}_j$ and $\mathcal{G}'_j$ as a phasor on a unit circle. Right: sequence used to construct a symmetrized sequence.

shall refer to this as symmetrization. This would entail the situation shown in 14(a) where the grating $\mathcal{G}_j = 1 + e^{i\tau_j\omega_j} + e^{i2\tau_j\omega_j} + \cdots + e^{i(F-1)\tau_j\omega_j}$ is followed by the grating, $\mathcal{G}'_j = e^{i(F-1)\tau_j\omega_j} + e^{i(F-2)\tau_j\omega_j} + \cdots + 1$ in a total of $2L$ cycles. Fig. 14 shows example of how this can be obtained in practice, for $F=3$. This yields the propagator,

$$
\begin{aligned}
U &= e^{itH_1}\left(e^{i\tau_j H_2} e^{itH_1} e^{-i\tau_j H_2}\right)\left(e^{i(2\tau_j)H_2} e^{itH_1} e^{-i(2\tau_j)H_2}\right) \\
&\times \left(e^{i(2\tau_j)H_2} e^{itH_1} e^{-i(2\tau_j)H_2}\right)\left(e^{i\tau_j H_2} e^{itH_1} e^{-i\tau_j H_2}\right) e^{itH_1} \\
&= \left[e^{itH_1} e^{i\tau_j H_2}\right]^{F-1} \times e^{i(2t)H_1} \times \left[e^{-i\tau_j H_2} e^{itH_1}\right]^{F-1}, \qquad (11)
\end{aligned}
$$

which yields the desired effective Hamiltonian for filtered polarization. Since now the approximation is valid to second order in the Magnus expansion, the symmetrized sequence is far more robust to fluctuations in the driving power $\Omega$ during cross-polarization. Power fluctuations can be as large as 5% of the drive amplitude [**?** **?** ], thus it is critical that the filtering action is invariant to the exact value of $\Omega$. Indeed, if one considers only the zeroth order average Hamiltonian, a slight variation in $\Omega$ should not affect the position of the grating maxima $\mathcal{G}_j$, which should following $\tau_j = 2m\pi/\omega_j$ ideally just depend on the delay periods $\tau$. However, due to the presence of non vanishing higher order terms in the Magnus expansion, we find that there is in fact a dependence on the $\mathcal{G}_j$ maxima on $\Omega$ (see 15).

In contrast, the symmetrized sequence is robust against variations on the value of $\Omega$. Thus, even if the Hartmann-Hahn condition is not exactly satisfied the filtering action is unaffected and the positions of the $\mathcal{G}_j$ maxima are determined only by the timing $t_g$. In addition to improved robustness, this could facilitate the experiments, since one could just fix $\Omega = \omega_L$ and achieve the selective polarization transfer by sweeping the filter time $t_g$. The tradeoff for this higher robustness is that one needs twice the number of cycles (and hence twice the experimental time) to achieve the same linewidth as in the unsymmetrized case (15).

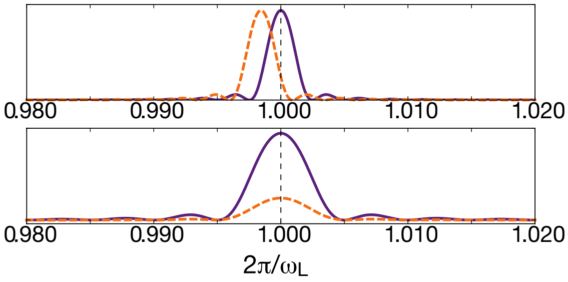


Figure 15: Effects of symmetrization of the selective Hartmann-Hahn sequence. We compare the unsymmetrized (top panel) and symmetrized (lower panel) sequences for an NV coupled to a single spin with Larmor frequency $\omega_L$. The spin lock frequencies were $\Omega = 0.95\omega_L$ (orange dashed line) and $\Omega = \omega_L$ (violet line). Under the unsymmetrized sequence, there is a shift in the resonance peak when $\Omega \neq \omega_L$. This shift is due to higher order terms in the Magnus expansion, and cannot be explained by the simple zero-order approximation based grating function filter in Eq. 8 of the main text. The symmetrized sequence, on the other hand, has a vanishing first order term, and is immune to shifts in $\Omega$ and hence is robust under power fluctuations.

## 5 Comparison with other sensing schemes

We compare different NV-based sensing methods that have been proposed. This highlight the advantages of the proposed cross-polarization based sensing protocol. Not only can the method achieve high frequency resolution, as it incorporates the filtering effects of dynamical-decoupling based sensing, but it also offers other benefits. Specifically, it allows the simultaneous application of homonuclear decoupling sequences on the nuclear spins and importantly it enables acquiring 2D spectra that encode information about the nuclear spins interconnectivity.

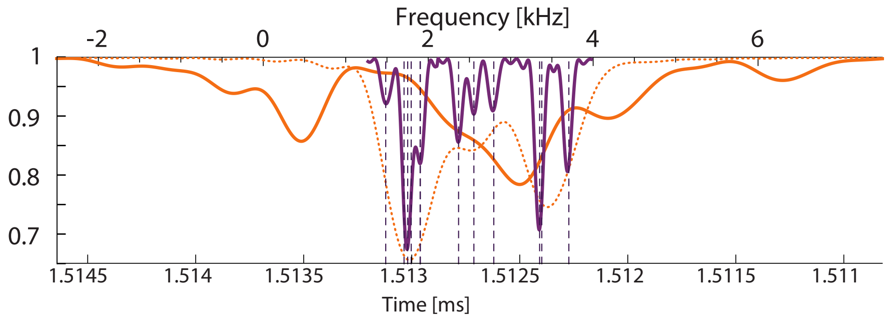


Figure 16: Comparison of DD-based sensing with filtered cross-polarization sensing methods. Even assuming very good performances of the dynamical decoupling sequence (1200 pulses and $T_2 > 1.5$ms) and no effect of the spin couplings (dotted line), the frequency resolution is not as good as for the filtered cross-polarization scheme (orange line). When spin couplings are taken into account, the spectrum broadens further (thick solid line) preventing the spatial position recontruction.

## 6 Geometrical pictures of the sensing schemes

An intuitive understanding of the (filtered) sensing schemes can be gained from a geometric picture of the relevant evolution. In this section we first present this picture for the dynamical-decoupling based NV sensing, considering in particular the effect of varying the two parameters under the experimenter's control – the period between pulses $\tau_j$ and the number of cycles $L$. We then present an analogous analysis for the filtered cross-polarization sensing.

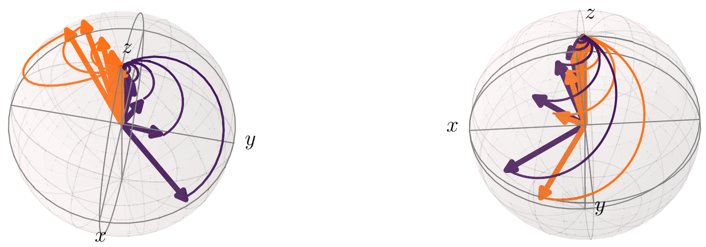


Figure 17: Bloch sphere representation of the dynamical-decoupling based nuclear sensing sequence. (a) Evolution of one nuclear spin in the $|0\rangle$ (orange) and $|1\rangle$ (violet) subspaces of the electron spin, under the action of $F$ cycles. These effective propagator under such cycles can be considered as concatenated rotations, and the effective nuclear axes move apart with increasing $F$. The final signal contrast depends on $\cos\Phi$, where $\Phi$ is the angle between the two axes. Hence increasing $F$ increases the sensing SNR. Note that the trajectories shown represent the path traversed on the Bloch sphere given the propagator $e^{-iH_at}e^{-2iH_bt}e^{-iH_at}$ ($\{a,b\} = \{0,1\}$) and serves as a guide to the eye. (b) Trajectories of different nuclear spins. We consider two nuclear spins separated by 1% in their effective Larmor frequencies and consider the effective nuclear axes (orange and violet arrows) in the $|0\rangle$ subspace for $F$ cycles of the sequence. As F increases, the two arrows move farther apart, signaling that the resolution increases with increasing $F$.

### 6.1 Dynamical decoupling-based spin sensing

Dynamical decoupling sensing sequence works by creating two different axes of rotation of the nuclear spins, conditioned on the $|0\rangle$ or $|1\rangle$ subspace of the NV. Indeed, in the rotating frame of the NV, the Hamiltonian can be written as $H = H = |0\rangle\langle 0| H_0 + |1\rangle\langle 1| H_1$, where $H_0 = \omega_L \sum I_{zj}$ and $H_1 = \sum_j [(\omega_L + A_j)I_{zj} + B_{\perp,j} I_{\perp,j}]$. Consider for simplicity a single nuclear spin under a periodic dynamical decoupling (PDD) sequence. The dips in the signal occur when the PDD pulses are separated by $\tau = (2m+1)\pi/\omega_L$. For $A, B_\perp \ll \omega_L$ this effectively generates $\pi$ rotations about different effective nuclear axes, as shown on a Bloch sphere in Fig (17).

Consider the nuclear evolution in the $|0\rangle$ subspace of the NV. The propagator is then,

$$\begin{aligned} U_1^0 &= \exp(iH_1\tau_j)\exp(iH_0\tau_j)\exp(iH_1\tau_j) \approx \exp(i\pi\hat{H}_1)\exp(i\pi\hat{H}_0)\exp(i\pi\hat{H}_1) \\ &= -\exp(i\pi\hat{H}_1)\exp(i\pi\hat{H}_0)\exp(-i\pi\hat{H}_1) = -\exp(i\pi\hat{H}_1') \end{aligned}$$

where the operators with the hat refer to normalized nuclear rotation axes, and we used $e^{i(2\pi)\hat{H}_1} = -1$ in the last line. Here $H_1' = e^{i\pi H_1} H_0 e^{-i\pi H_1}$ is the effective axis formed by rotating $H_0$ around the generator $H_1$ by $\pi$ radians. In the $|1\rangle$ subspace one gets the same expression but with the $H_0, H_1$ reversed.

$$U_1^1 = \exp(i\pi\hat{H}_0)\exp(i\pi\hat{H}_1)\exp(-i\pi\hat{H}_0) = -\exp(i\pi\hat{H}_0') \tag{12}$$

Similarly if one considers now the concatenated rotation,

$$U_2^0 = \exp(iH_1'\tau_j)\exp(iH_0\tau_j)\exp(iH_1'\tau_j) \approx \exp(i\pi\hat{H}_1'') \tag{13}$$

where now $H_1'' = e^{i\pi H_1'} H_0 e^{-i\pi H_1'}$ is the effective axes formed by rotating $H_0$ around the generator $H_1'$ by $\pi$ radians. Hence with each concatenated rotation, the effective nuclear spin rotation axes in the two subspaces move further out (see 17). This leads to the increasing dispersion between the two nuclear axes – and as one increases the number of cycles $n$ these axes move apart further, and the final signal depends on the cosine of the angle between these two final axes. Hence increasing $n$ leads to higher SNR.

One can observe that the frequency resolution improves as the number of cycles is increased (Fig. 17(b)). Consider two nuclear spin axes in the $|0\rangle$ subspace, and as $n$ increases the relative angle between them gets magnified. This leads to higher resolution. Resolution can also be improved by going to higher multiples of $\pi/\omega_L$ for the same reason –any difference between the two angles get magnified (because in effect one is close to a $\pi$ rotation but not exactly $\pi$).

The frequency resolution is ultimately limited by the intrinsic NMR linewidth of the target nuclear spins. In principle, one could embed a homonuclear dynamical decoupling sequence (such as wahuha [**?** ] or mrev8 [**?** ]) in the sensing scheme. In practice, this might result quite difficult. Ideally one would want the nuclear spin system to evolve under the Hamiltonians $H_0$ and $H_1$ during alternating time periods. Because of spin couplings, the Hamiltonians are instead $H_0' = H_0 + H_0^{(nn)}$ and $H_1' = H_0 + H_1^{(nn)}$, where $H_i^{(nn)}$ describes the nuclear spin-spin interaction (which might be different in the two NV manifolds [**?** ]). A homonuclear sequence during each time period $\tau$ could average this Hamiltonian to zero. However this implies that the nuclear spin pulse separation should be $\delta t \leq \tau/6 = (2m+1)\pi/(6\omega_L)$ and the nuclear spin pulse duration itself $t_p$ should be at least 1-2 times smaller. For small $m$, this condition would require violating the rotating wave approximation for the nuclear spin pulses. We would need large $m \geq 100$ to be able pulse on the nuclear spins (which might not be possible given the NV coherence time) and even then, the required driving strength might exceed what is experimentally feasible.

We note that this problem does not arise with cross-polarization based sensing, since there is no requirement to achieve a full decoupling cycle in a given short time $\tau$.

### 6.2 Filtered cross-polarization spin sensing

We now consider a similar geometric picture for the filtering effects of cross polarization protocol that causes the narrower linewidth. In contrast to the previous section, cross-polarization under spin locking involves two spins and cannot be directly visualized on a Bloch sphere. To aid the geometric visualization of the polarization exchange between the NV and a nuclear spin we employ the $\{\Sigma, \Delta\}$ Hamiltonian decomposition [**?** **?** ]. For simplicity, let us consider the Hamiltonian,

$$H = \omega S_z + \omega_L I_z + B S_x I_x \tag{14}$$

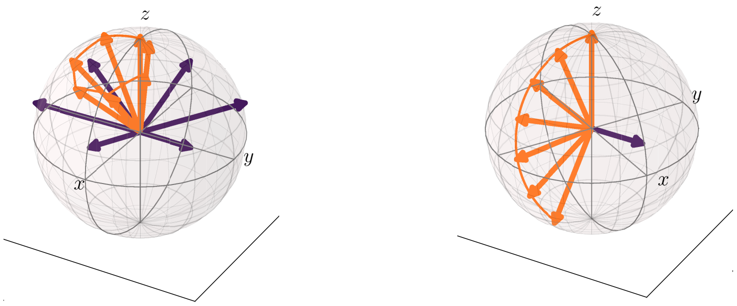


Figure 18: Bloch spheres showing the filtering action in the $\Delta$ subspace. The violet arrows are the Hamiltonians $H_\Delta$ and the orange arrows trace the evolution of the spin vector $S^\Delta$. (a) Non-resonant case of the filter i.e. when the period $\tau \neq 2m\pi/\omega_L$. As the vector $\Sigma(0) = S_z^\Delta$ starts tipping, the Hamiltonian gets effectively rotated after every cycle of the sequence, and if L is large enough the spin vector returns to the north pole without tipping, leading to no polarization transfer. Hence the filtering action physically exploits the coherence on the nuclear spin. (b) Resonant case when $\tau \approx 2m\pi/\omega_L$. Now the Hamiltonian gets rotated in such a manner that it always returns to the same position on the Bloch sphere after every cycle. The effect is that the tipping of the spin vector adds up coherently, and there is effective polarization transfer.

which is the active part of the Hartmann-Hahn Hamiltonian in the frame of reference that is tilted with respect to the NV spin locking frame. In the $\{\Sigma, \Delta\}$ basis defined by,

$$S_z^\Sigma = \tfrac{1}{2}(S_z + I_z) \qquad S_z^\Delta = \tfrac{1}{2}(S_z - I_z)$$

$$S_x^\Sigma = \tfrac{1}{2}(S^+I^+ + S^-I^-) \quad S_x^\Delta = \tfrac{1}{2}(S^+I^- + S^-I^+)$$

$$S_y^\Sigma = \tfrac{1}{2i}(S^+I^+ - S^-I^-) \quad S_y^\Delta = \tfrac{1}{2i}(S^+I^- - S^-I^+)$$

this Hamiltonian can be written as $H = H_\Sigma + H_\Delta$ with

$$H_\Sigma = (\omega_L + \omega)S_z^\Sigma + BS_x^\Sigma = \omega^\Sigma \left[S_z^\Sigma \cos(\vartheta_\Sigma) + S_x^\Sigma \sin(\vartheta_\Sigma)\right]$$

$$H_\Delta = (\omega_L - \omega)S_z^\Delta + BS_x^\Delta = \omega^\Delta \left[S_z^\Delta \cos(\vartheta_\Delta) + S_x^\Delta \sin(\vartheta_\Delta)\right]$$

where $\omega^\Sigma = \sqrt{(\omega_L + \omega)^2 + B^2}$, $\omega^\Delta = \sqrt{(\omega_L - \omega)^2 + B^2}$ and $\sin(\vartheta_{\Sigma,\Delta}) = B/\omega^{\Sigma,\Delta}$ . In this basis, the initial state is fully polarized along the north pole in both subspaces,

$$\Sigma(0) = S_z = S_z^\Sigma + S_z^\Delta$$

Close to the Hartmann-Hahn matching condition, the $\Sigma$ subspace does not evolve and full polarization transfer occurs when the $S_z$ operator starting at the north pole ends up at the south pole of the $\Delta$-space Bloch sphere (see 18).

The filtering action of the sequence can now be visualized in this basis, focusing on the $\Delta$ subspace. For a sequence of alternating period of evolution under the polarization and gradient Hamiltonians, we achieve an effective polarization Hamiltonian modulated by the grating. In the $\Delta$ subspace, this Hamiltonian for instance has the form $H_\Delta = (\omega_L - \omega)S_z^\Delta + B\cos\vartheta S_x^\Delta + B\sin\vartheta S_y^\Delta$. If the filter is off-resonance, $\vartheta \neq 2\pi$ and the axes of the effective rotation keeps changing at each cycle of the sequence, thus the state $S_z^\Delta$ is unable to flip completely (18(a)). For instance, if $\vartheta = \pi$ the effective Hamiltonians in alternate cycles is $\omega S_z + \omega_L I_z \pm BS_xI_x$, and polarization is fed into and removed from the nuclear spins in alternate cycles. In contrast when $\vartheta = 2\pi$, the filter is resonant and the action of every cycle adds coherently leading to an inversion in $\Delta$ subspace and polarization transfer (Fig. 18(b)).
